# Supplementary material for: 360+x: A Panoptic Multi-modal Scene Understanding Dataset
Source: arXiv:2404.00989 source file (2024-04-08)
Supplement: Supplementary file 1 [file dataset_comparison.tex]

\begin{table*}[!t]
	\caption{ \textbf{Datasets comparison.} FV V: Front-view Video, \du~V:\du~Video, Ego M V: Egocentric Monocular Video, Ego S V: Egocentric Stereo Video, Normal A: Normal Audio, Directional A: Directional Audio, V: Video, A: Audio, AV: Audio-visual events.}
    % \hspace{0.2pt}
	\small
	\centering
	\setlength{\tabcolsep}{4pt}
 % \hspace{-1cm}   % Modify here to shift the table horizontally....................
    \resizebox{1\textwidth}{!}{
    \begin{tabular}{l|c|c|c|c|c|c|c|c|c|c}
     \toprule
     \multirow{2}{*}{Dataset}  & \multicolumn{7}{c|}{Modalities} &\multirow{2}{*}{Avg Duration}& \multirow{2}{*}{Annotations}& \multirow{2}{*}{Multiple Events} \\
     % &Front-view Video&\du Video&Egocentric Video&Normal Audio&Normal Audio&Directional Audio& GPS Data&&&&&&\\
     &FV V&\du~V&Ego M V&Ego S V
&Normal A&Directional A& GPS \\
     \midrule
    UCF101~\cite{soomro2012ucf101}&\cmark&\xmark&\xmark&\xmark&\cmark&\xmark&\xmark&7.21 s&V&\xmark\\
    Kinetics~\cite{kay2017kinetics}&\cmark&\xmark&\xmark&\xmark&\xmark&\xmark&\xmark&10 s&V&\xmark\\
    
    HMDB51~\cite{Kuehne11}&\cmark&\xmark&\xmark&\xmark&\xmark&\xmark&\xmark&3 s&V&\xmark\\
    
    ActivityNet~\cite{caba2015activitynet}&\cmark&\xmark&\xmark&\xmark&\cmark&\xmark&\xmark&2 min&V&\cmark\\
    
    EPIC-Kitchen~\cite{damen2018scaling}&\cmark&\xmark&\xmark&\xmark&\cmark&\xmark&\xmark&7.6 min&V&\xmark\\
    Ego4D~\cite{grauman2022ego4d}&\cmark&\xmark&\xmark&\xmark&\cmark&\xmark&\cmark&8 min&AV&\cmark\\

    \midrule
    Ours&\cmark&\cmark&\cmark&\cmark&\cmark&\cmark&\cmark&6 min&AV&\cmark\\
% ---------------------- Color ------------------------------
   % \midrule

     \bottomrule
    \end{tabular}
    }
    
\vspace{-0.1cm}
\label{tab:dataset comparison}
\end{table*}

% UCF101	√	❌	❌	❌	√	❌	❌	5	2500	101	7.21 s	V	❌
% Kinetics	√	❌	❌	❌	❌	❌	❌	-	306245	400	10 s	A	❌
% HMDB51	√	❌	❌	❌	❌	❌	❌	-	3312	51	-	V	❌
% ActivityNet	√	❌	❌	❌	√	❌	❌	-	19994	200	-	V	❌
% EPIC	√	❌	❌	❌	√	❌	❌	32	432	149	7.6 min	V	❌
% Ego4D	√	❌	❌	❌	√	❌	√	14	≈27525	-	8min	AV	√
													
% Ours	√	√	√	√	√	√	√	22	400	27		AV	√
