# Supplementary material for: 360+x: A Panoptic Multi-modal Scene Understanding Dataset
Source: arXiv:2404.00989 source file (2024-04-08)
Supplement: Supplementary file 2 [file ssl+tal.tex]

\begin{table}
\begin{minipage}{.39\textwidth}
% \begin{table*}
	\centering
	\caption{Models pre-trained with different self-supervise methods were tested on video classification. The methods using all three video types together.}
 \vspace{2mm}
%     % \hspace{0.2pt}
% 	\small
% 	% \setlength{\tabcolsep}{4pt}
\resizebox{\textwidth}{!}{
    \begin{tabular}{@{}c|c|c@{}}
     \toprule
    Pre-trained Method &  Modalities  &  Mean Precision (\%) $ \ \pm\  $ STD \\
      \midrule
      \multirow{3}{*}{From Scratch} %& \multirow{3}{*}{360$^{\circ}$  + Front +  Binocular}
      &   V   &          $ 0.72 \ \pm \ 0.027  $  \e{0.00} \\  
      & V + A &        $ 0.83\  \pm\  0.027  $   \e{0.00}   \\
      & V + A + D  &   $ 0.89 \ \pm \ 0.022  $  \e{0.00}    \\
      \midrule
      \multirow{3}{*}{Video Pace} %&& \multirow{3}{*}{360$^{\circ}$  + Front +  Binocular}
      &   V   &          $ 0.80 \ \pm \ 0.025  $   \p{0.08} \\  
      & V + A &        $ 0.86\  \pm\  0.023  $    \p{0.03}  \\
      & V + A + D  &   $ 0.93 \ \pm \ 0.020  $     \p{0.04} \\
      \midrule
    \multirow{3}{*}{Video Clip Order} %&& 
    % \multirow{3}{*}{360$^{\circ}$  + Front +  Binocular}
      &   V   &          $ 0.82 \ \pm \ 0.024  $   \p{0.10}\\  
      & V + A &        $ 0.87\  \pm\  0.023  $    \p{0.04}  \\
      & V + A + D  &   $ 0.93 \ \pm \ 0.019  $     \p{0.04} \\
      \midrule
     \multirow{3}{*}{\makecell[c]{   Video Pace\\+\\Video Clip Order    }}  
    % \multirow{3}{*}{360$^{\circ}$  + Front +  Binocular} 
      &   V   &          $ 0.88 \ \pm \ 0.022  $   \p{0.16} \\  
      &  V + A &        $ 0.91\  \pm\  0.021  $   \p{0.08}   \\
      &  V + A + D  &   $ 0.96 \ \pm \ 0.015  $     \p{0.07} \\
      % \midrule
     \bottomrule
    \end{tabular}
    }
% \vspace{-0.1cm}
\label{tab:ssl}
% \end{table*}
\end{minipage}%
\hfill
\begin{minipage}{.59\textwidth}
% \begin{table*}
	\centering
	 \caption{Comparison between supervised pre-trained extractors with SSL pre-trained counterparts for temporal action localization.}
 \vspace{2mm}
%     % \hspace{0.2pt}
% 	\small
% 	% \setlength{\tabcolsep}{4pt}
% % \hspace*{-1.0cm}
\resizebox{\textwidth}{!}{
    \begin{tabular}{@{}c|c|c|c|c|c@{}}
     \toprule
      Pre-training Method &   Modalities  & mAP$@$0.5 & mAP$@$0.75 & mAP$@$0.95& Avg.  \\
      \midrule
    \multirow{3}{*}{\makecell[c]{Supervised
    Baseline\\Extractors }} 
       & V   &           $18.4 $    & $ 10.8$    &  $3.3$   &  $10.8$\e{0.00}    \\  
       & V + A&     $23.6$      &  $16.2$    & $5.2$   &  $15.0$\e{0.00}  \\         
       & V + A + D  & $25.9$     &   $17.8$                   &   $5.3$      &   $16.3$\e{0.0}  \\
       \midrule
      \multirow{3}{*}{\makecell[c]{  Video Pace     }} 
       & V   &     $ 24.4   $            &   $14.9$                 &    $6.6$  & $15.3$\p{4.5} \\  
       & V + A&     $28.7  $        &   $18.2$                  &    $7.1$   &  $18.0$\p{3.0} \\  
       & V + A + D  & $30.9$     &   $20.8$                   &     $7.5$  & $19.7$\p{3.4}  \\
        \midrule
    \multirow{3}{*}{\makecell[c]{  Video Clip Order     }} 
       & V   &        $ 24.6   $            &   $15.2$         &    $6.7$  & $15.5$\p{4.7} \\  
       & V + A&     $ 28.5  $        &   $18.0$              &    $7.0$   &  $17.8$\p{2.8} \\  
       &  V + A + D  & $30.2$     &   $19.9$                  &   $7.3$  & $19.1$\p{2.8}  \\
        \midrule 
    \multirow{3}{*}{\makecell[c]{  Video Pace\\+\\Video Clip Order       }} 
       & V   &     $ 25.5   $            &   $18.0$               &    $7.4$  & $17.0$\p{6.2} \\  
       &  V + A&     $29.4  $        &   $20.2$                  &    $8.0$   &  $19.2$\p{4.2} \\  
       &  V + A + D  & $31.1$     &   $20.5$                     &    $8.4$  & $20.0$\p{4.7}  \\
     \bottomrule
    \end{tabular}
    }
% \vspace{-0.1cm}
\label{tab:tal2}
% \end{table*}
\end{minipage}

\end{table}
