# Supplementary material for: 360+x: A Panoptic Multi-modal Scene Understanding Dataset
Source: arXiv:2404.00989 source file (2024-04-08)
Supplement: Supplementary file 3 [file tal.tex]

% \hspace{-2cm}

\begin{table*}[!t]
	 \caption{\textbf{Temporal action localization result.} Extractors were trained on video classification with different datasets.  The mAP$@$0.5 represents the mean average precision at a threshold of $0.5$. }

    % \hspace{0.2pt}
	% \small
	\centering
	% \setlength{\tabcolsep}{4pt}

% \hspace*{-1.2cm}
\resizebox{\textwidth}{!}{
    \begin{tabular}{@{}c|cc|c|c|c|c|c@{}}
     \toprule
 
    Extractors & \multicolumn{2}{c|}{Pre-trained Datasets}   & Modalities  & mAP$@$0.5 & mAP$@$0.75 & mAP$@$0.95& Avg.  \\
      \midrule
      
       \multirow{3}{*}{\makecell[c]{  Baseline \\ Extractors   }}  &  \multirow{3}{*}{\makecell[c]{ Video: \\Audio: \\Directional: }}  &  \multirow{3}{*}{\makecell[c]{  Kinetics 400 \cite{kay2017kinetics}\\AudioSet \cite{audioset}\\ - }}  
       & V   &           $18.4 $    & $ 10.8$    &  $3.3$   &  $10.8$\e{0.00}    \\  
       & & & V + A&     $23.6$      &  $16.2$    & $5.2$   &  $15.0$\e{0.00}  \\  
       & & & V + A + D  &  ---  & --- & ---  & ---  \\ 
      \midrule
      
     \multirow{3}{*}{\makecell[c]{  Pre-trained \\ on \textit{360+x}     }} & \multirow{3}{*}{\makecell[c]{ Video: \\Audio: \\Directional: }}  &  \multirow{3}{*}{\makecell[c]{  \textit{360+x}\\\textit{360+x}\\\textit{360+x}}}
       & V   &     $ 25.8   $            &   $17.7$                 &    $6.8$  & $16.8$\p{6.00} \\  
       & & & V + A&     $30.1  $        &   $20.4$                  &    $7.5$   &  $19.3$\p{4.30}\\  
       & & & V + A + D  & $\boldsymbol{32.4}$     &   $\boldsymbol{21.1}$      &   $\boldsymbol{7.8}$  & $\boldsymbol{20.4}$  \\
     \bottomrule
    \end{tabular}
    }
\vspace{-0.1cm}
\label{tab:tal}
\end{table*}

% \hspace{-2cm}

% \begin{table*}[!ht]
% 	 \caption{\textbf{Temporal action localization result.} The feature extractors are pretrained using \textit{video pace + clip order} method on video classification task.}
%  % \multirow{3}{*}{360$^{\circ}$  + Front +  Binocular}
%     \hspace{0.2pt}
% 	\small
% 	\centering
% 	\setlength{\tabcolsep}{4pt}

% \hspace*{-1.2cm}
%     \begin{tabular}{c|cc|c|c|c}
%      \toprule
 
%     Pre-trained Method & \multicolumn{2}{c}{Pre-trained Datasets}   & Modalities  & Top-1 Accuracy (\%) & Top-5 Accuracy (\%) \\
%       \midrule
      
%        \multirow{3}{*}{\makecell[c]{  Supervised with \\ Video Classification    }}  &  \multirow{3}{*}{\makecell[c]{ Video: \\Audio: \\Directional: }}  &  \multirow{3}{*}{\makecell[c]{  Kinetics 400 \cite{carreira2018quo}\\AudioSet \cite{audioset}\\360+X}}  
%       & V   &                        \\  
%        & & & V + A&                        \\  
%        & & & V + A + D  & -  & -\\
%       \midrule
      
%      \multirow{3}{*}{\makecell[c]{  Supervised with \\ Video Classification    }} & \multirow{3}{*}{\makecell[c]{ Video: \\Audio: \\Directional: }}  &  \multirow{3}{*}{\makecell[c]{  360+X\\360+X\\360+X}}
%        & V   &                        \\  
%        & & & V + A&                        \\  
%        & & & V + A + D  & -  & -\\

%      \bottomrule
%     \end{tabular}
% \vspace{-0.1cm}
% \label{tab:tal}
% \end{table*}
