# Supplementary material for: 360+x: A Panoptic Multi-modal Scene Understanding Dataset
Source: arXiv:2404.00989 source file (2024-04-08)
Supplement: Supplementary file 4 [file temporal.tex]

% \begin{table*}[!h]
%     \caption{Temporal Labels Dictionary}
%     \small
%     \centering
%     \setlength{\tabcolsep}{4pt}
%     \begin{tabular}{c|c}
%      \toprule
%     Temporal Segmentation Label & Duration Percentage \\
%       \midrule
%       walking & 20.95% \\
%       speaking & 18.07% \\
%       operating phone & 17.54% \\
%       eating & 8.89% \\
%       playing instrument & 4.46% \\
%       firework & 3.97% \\
%       playing & 2.59% \\
%       preparing food & 2.29% \\
%       reading & 1.94% \\
%       operating computer & 1.85% \\
%       photographing & 1.85% \\
%       drinking & 1.75% \\
%       dressing & 1.71% \\
%       housekeeping & 1.63% \\
%       workout & 1.56% \\
%       farming & 1.55% \\
%       moving things & 1.03% \\
%       hygiene practices & 0.94% \\
%       cooking & 0.83% \\
%       pouring & 0.68% \\
%       laughing & 0.50% \\
%       sitting & 0.44% \\
%       playing card games & 0.43% \\
%       dancing & 0.32% \\
%       driving & 0.30% \\
%       clapping & 0.30% \\
%       opening & 0.30% \\
%       selling & 0.26% \\
%       coughing & 0.25% \\
%       standing & 0.23% \\
%       flashing & 0.18% \\
%       pushing & 0.16% \\
%       running & 0.09% \\
%       cleaning & 0.09% \\
%       smoking & 0.03% \\
%       Assisting & 0.03% \\
%       alarming & 0.01% \\
%       smelling & 0.00% \\
%      \bottomrule
%     \end{tabular}
% \label{tab:temporal}
% \end{table*}

\begin{table}[h]
\centering
\begin{tabular}{|l|}
\hline
Temporal Segmentation Label \\ \hline
walking \\ \hline
speaking \\ \hline
operating phone \\ \hline
eating \\ \hline
playing instrument \\ \hline
firework \\ \hline
playing \\ \hline
preparing food \\ \hline
reading \\ \hline
operating computer \\ \hline
photographing \\ \hline
drinking \\ \hline
dressing \\ \hline
housekeeping \\ \hline
workout \\ \hline
farming \\ \hline
moving things \\ \hline
hygiene practices \\ \hline
cooking \\ \hline
pouring \\ \hline
laughing \\ \hline
sitting \\ \hline
playing card games \\ \hline
dancing \\ \hline
driving \\ \hline
clapping \\ \hline
opening \\ \hline
selling \\ \hline
coughing \\ \hline
standing \\ \hline
flashing \\ \hline
pushing \\ \hline
running \\ \hline
cleaning \\ \hline
smoking \\ \hline
Assisting \\ \hline
alarming \\ \hline
smelling \\ \hline
\end{tabular}
\caption{List of Temporal Segmentation Labels}
\end{table}
