# Supplementary material for: 360+x: A Panoptic Multi-modal Scene Understanding Dataset
Source: arXiv:2404.00989 source file (2024-04-08)
Supplement: Supplementary file 6 [file supp_teaser.tex]

\begin{strip}
\centering
\vspace{-0.5cm}
\vstretch{1.1}{\includegraphics[width=\textwidth]{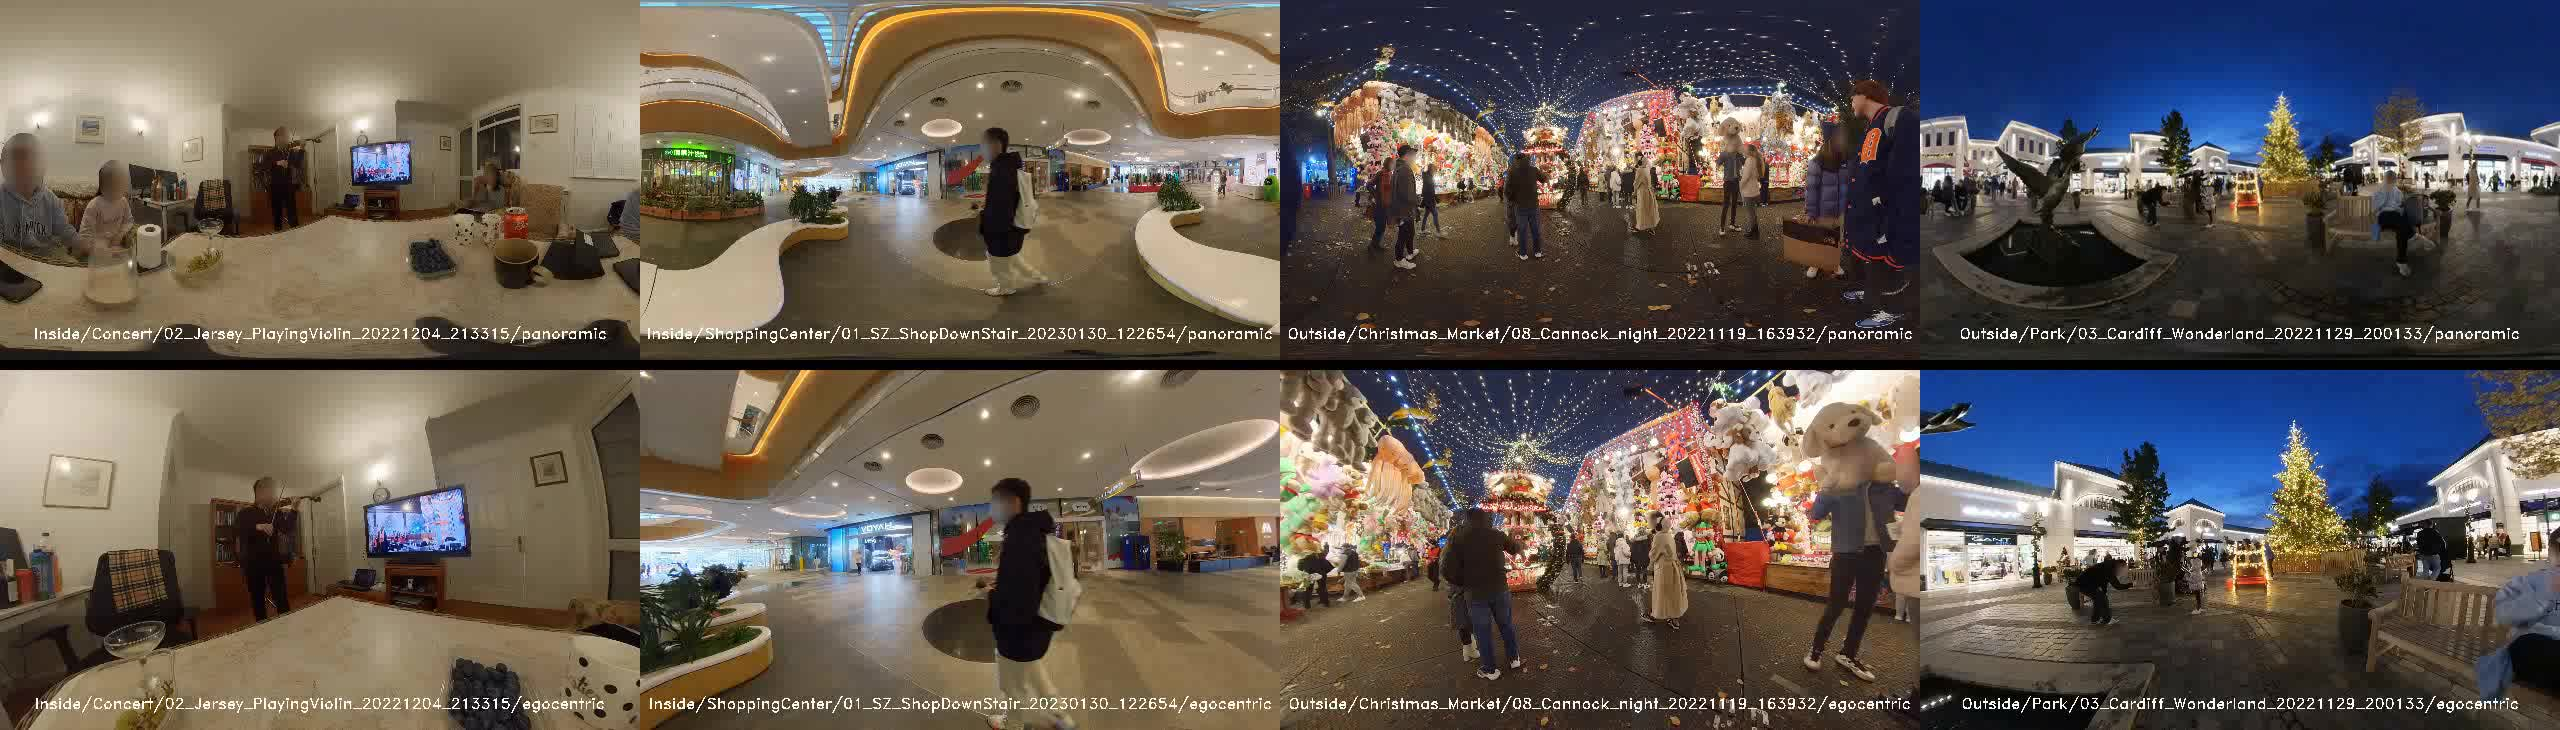}}
\captionof{figure}{Example indoor/outdoor front view videos.}
\label{fig:supp_teasor}
\end{strip}
