# Supplementary material for: 360+x: A Panoptic Multi-modal Scene Understanding Dataset
Source: arXiv:2404.00989 source file (2024-04-08)
Supplement: Supplementary file 7 [file cls.tex]

% \begin{table*}[!t]
\begin{wraptable}{r}{0.6\textwidth}
	% \caption{ \textbf{Video classification results.} The results obtained using only the \du view serve as a baseline for each respective modality combination. V:Video, A:Audio, D:Directional audio time delay.}
	\caption{ \textbf{Video classification results.} V: Video, A: Audio, D: Directional audio.}
    % \hspace{0.2pt}
	\small
	\centering

\resizebox{0.6\textwidth}{!}{
    \begin{tabular}{c|c|c}
     \toprule
 
     Selected Video Views  & Modalities  & Mean Precision (\%) $ \ \pm\  $ STD \\
      \midrule
      % \multicolumn{3}{c}{Single Video Type} \\
      % \midrule
     \multirow{3}{*}{360$^{\circ}$ View Only}
      & V   &       $0.55\ \pm\  0.027 $       \e{0.00}        \\  
      & V + A &     $0.72\  \pm\  0.027 $      \e{0.00}         \\
      & V + A + D  &   $0.77\  \pm\  0.022 $   \e{0.00}       \\
      \midrule

      \multirow{3}{*}{Front View Only}
      & V   &       $0.49\  \pm \ 0.041$  \m{0.06}       \\  
      & V + A &       $0.61\  \pm \ 0.041$   \m{0.11}         \\
      & V + A + D  &   $0.75 \ \pm\  0.035$    \m{0.02}       \\
      \midrule

      \multirow{3}{*}{Binocular View Only}
      & V   &        $0.53\  \pm\  0.035$   \m{0.02}       \\  
      & V + A &       $0.64\  \pm\  0.031$      \m{0.08}     \\
      & V + A + D  &    $0.73\  \pm\  0.027$   \m{0.04}     \\
      \midrule

      \multirow{3}{*}{360$^{\circ}$ + Front}
      & V   &        $0.59\  \pm \   0.041 $ \p{0.04}    \\  
      & V + A &      $0.74\  \pm\  0.022  $   \p{0.07}       \\
      & V + A + D  &   $0.79\  \pm\  0.044$   \p{0.02}     \\
      \midrule

      \multirow{3}{*}{360$^{\circ}$ + Binocular} 
      & V   &       $0.65 \ \pm \   0.035   $ \p{0.10}   \\  
      & V + A &      $0.78\  \pm\  0.035   $   \p{0.06}       \\
      & V + A + D  &  $0.83\  \pm\  0.022   $    \p{0.06}     \\
      \midrule

      \multirow{3}{*}{360$^{\circ}$  + Front +  Binocular}
      & V   &          $ 0.72 \ \pm \ 0.027  $  \p{0.17} \\  
      & V + A &        $ 0.83\  \pm\  0.027  $   \p{0.11}   \\
      & V + A + D  &   $ \boldsymbol{0.89 \ \pm \ 0.022  }$     \p{0.12} \\

% ---------------------- Color ------------------------------
   % \midrule

     \bottomrule
    \end{tabular}
    }
\vspace{-0.1cm}
\label{tab:cls}
% \end{table*}
\end{wraptable}
