# Supplementary material for: 360+x: A Panoptic Multi-modal Scene Understanding Dataset
Source: arXiv:2404.00989 source file (2024-04-08)
Supplement: Supplementary file 8 [file ssl.tex]

\begin{table*}[!h]
	\caption{Models pre-trained with different self-supervise methods were tested on video classification. The methods using all three video types together.}
    % \hspace{0.2pt}
	\small
	\centering
	\setlength{\tabcolsep}{4pt}

    \begin{tabular}{c|c|c}
     \toprule
 
    Pre-trained Method &  Modalities  &  Mean Precision (\%) $ \ \pm\  $ STD \\
      \midrule

      \multirow{3}{*}{From Scratch} %& \multirow{3}{*}{360$^{\circ}$  + Front +  Binocular}
      &   V   &          $ 0.72 \ \pm \ 0.027  $  \e{0.00} \\  
      & V + A &        $ 0.83\  \pm\  0.027  $   \e{0.00}   \\
      & V + A + D  &   $ 0.89 \ \pm \ 0.022  $  \e{0.00}    \\
      \midrule
      
      \multirow{3}{*}{Video Pace} %&& \multirow{3}{*}{360$^{\circ}$  + Front +  Binocular}
      &   V   &          $ 0.80 \ \pm \ 0.025  $   \p{0.08} \\  
      & V + A &        $ 0.86\  \pm\  0.023  $    \p{0.03}  \\
      & V + A + D  &   $ 0.93 \ \pm \ 0.020  $     \p{0.04} \\
      \midrule

    \multirow{3}{*}{Video Clip Order} %&& 
    % \multirow{3}{*}{360$^{\circ}$  + Front +  Binocular}
      &   V   &          $ 0.82 \ \pm \ 0.024  $   \p{0.10}\\  
      & V + A &        $ 0.87\  \pm\  0.023  $    \p{0.04}  \\
      & V + A + D  &   $ 0.93 \ \pm \ 0.019  $     \p{0.04} \\
      \midrule

     \multirow{3}{*}{\makecell[c]{   Video Pace\\+\\Video Clip Order    }}  
    % \multirow{3}{*}{360$^{\circ}$  + Front +  Binocular} 
      &   V   &          $ 0.88 \ \pm \ 0.022  $   \p{0.16} \\  
      &  V + A &        $ 0.91\  \pm\  0.021  $   \p{0.08}   \\
      &  V + A + D  &   $ 0.96 \ \pm \ 0.015  $     \p{0.07} \\
      % \midrule

     \bottomrule
    \end{tabular}
\vspace{-0.1cm}
\label{tab:ssl}
\end{table*}
