# Supplementary material for: 360+x: A Panoptic Multi-modal Scene Understanding Dataset
Source: arXiv:2404.00989 source file (2024-04-08)
Supplement: Supplementary file 9 [file tal2.tex]

% \hspace{-2cm}

\begin{table*}[!t]
	 \caption{Comparison between supervised pre-trained extractors with SSL pre-trained counterparts for temporal action localization.}
    % \hspace{0.2pt}
	\small
	\centering
	\setlength{\tabcolsep}{4pt}

% \hspace*{-1.0cm}
    \begin{tabular}{c|c|c|c|c|c}
     \toprule
 
      Pre-training Method &   Modalities  & mAP$@$0.5 & mAP$@$0.75 & mAP$@$0.95& Avg.  \\
      \midrule
              
    \multirow{3}{*}{\makecell[c]{Supervised
    Baseline\\Extractors }} 
       & V   &           $18.4 $    & $ 10.8$    &  $3.3$   &  $10.8$\e{0.00}    \\  
       & V + A&     $23.6$      &  $16.2$    & $5.2$   &  $15.0$\e{0.00}  \\         
       & V + A + D  & $25.9$     &   $17.8$                   &   $5.3$      &   $16.3$\e{0.0}  \\

       \midrule
      
      \multirow{3}{*}{\makecell[c]{  Video Pace     }} 
       & V   &     $ 24.4   $            &   $14.9$                 &    $6.6$  & $15.3$\p{4.5} \\  
       & V + A&     $28.7  $        &   $18.2$                  &    $7.1$   &  $18.0$\p{3.0} \\  
       & V + A + D  & $30.9$     &   $20.8$                   &     $7.5$  & $19.7$\p{3.4}  \\
        \midrule

    \multirow{3}{*}{\makecell[c]{  Video Clip Order     }} 
       & V   &        $ 24.6   $            &   $15.2$         &    $6.7$  & $15.5$\p{4.7} \\  
       & V + A&     $ 28.5  $        &   $18.0$              &    $7.0$   &  $17.8$\p{2.8} \\  
       &  V + A + D  & $30.2$     &   $19.9$                  &   $7.3$  & $19.1$\p{2.8}  \\
        \midrule

    \multirow{3}{*}{\makecell[c]{  Video Pace\\+\\Video Clip Order       }} 
       & V   &     $ 25.5   $            &   $18.0$               &    $7.4$  & $17.0$\p{6.2} \\  
       &  V + A&     $29.4  $        &   $20.2$                  &    $8.0$   &  $19.2$\p{4.2} \\  
       &  V + A + D  & $31.1$     &   $20.5$                     &    $8.4$  & $20.0$\p{4.7}  \\
        % \midrule 

    % \multirow{3}{*}{\makecell[c]{  Video Pace\\+\\Video Clip Order       }} 
    % % & \multirow{3}{*}{ \makecell[c]{  Video Classification       } } 
    %    & V   &     $ 28.2   $            &   $19.7$                          &    $7.9$         & $18.6$\p{7.8} \\  
    %    &  V + A&     $33.8  $        &   $22.3$                             &    $8.7$           &  $21.6$\p{6.6}  \\  
    %    &  V + A + D  & $\boldsymbol{34.6}$     &   $\boldsymbol{22.8}$      &   $\boldsymbol{9.2}$  & $\boldsymbol{22.2}$\p{5.9}  \\
       
     \bottomrule
    \end{tabular}
\vspace{-0.1cm}
\label{tab:tal2}
\end{table*}
