# Supplementary material for: 360+x: A Panoptic Multi-modal Scene Understanding Dataset
Source: arXiv:2404.00989 source file (2024-04-08)
Supplement: Supplementary file 10 [file dataset_analysis.tex]

\begin{figure}

\begin{subfigure}[t]{\textwidth}
  % \hspace{-1.3cm}  
  \includegraphics[width=1\linewidth]{img/analysis/scenes_time.png} 
   \caption{Video duration of inside and outside scenes.}
   \label{fig:time length}
\end{subfigure}

    \centering 

  \begin{subfigure}[b]{0.5\textwidth}
     % \hspace{-0.9cm}
     \includegraphics[width=\textwidth]{img/analysis/seg_tree.png}
    % \hspace{-0.3cm}
    \caption{Hierarchical distribution visualization of the temporal segmentation categories. }
    \label{fig:tsl}
  \end{subfigure}
  \hfill
  \begin{subfigure}[b]{0.48\textwidth}
    \includegraphics[width=\textwidth]{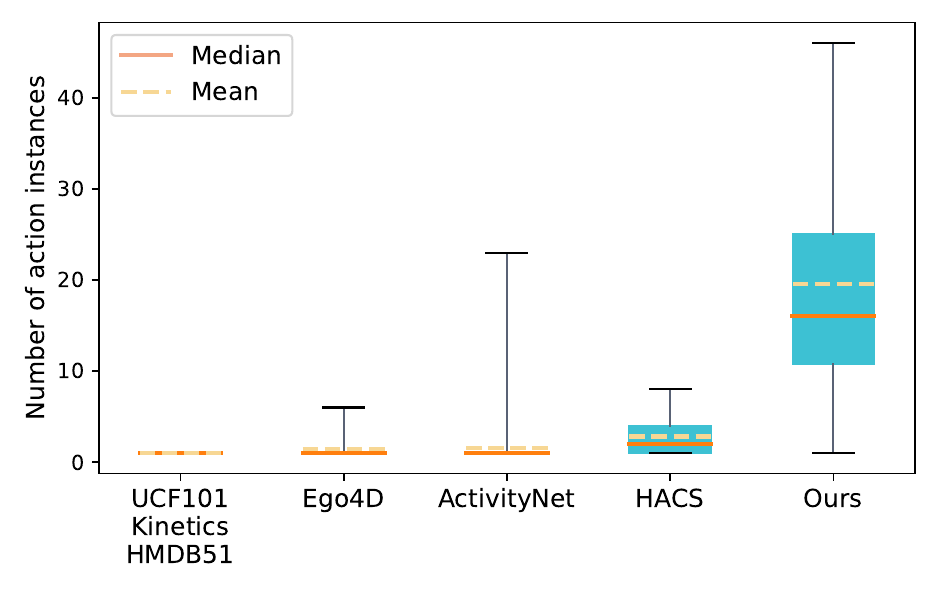}
    \caption{Distribution comparison of the number of action instances per video between existing datasets (e.g. UCF101 \cite{soomro2012ucf101}, Kinetics \cite{kay2017kinetics}, HMDB51 \cite{Kuehne11}, Ego4D \cite{grauman2022ego4d}, ActivityNet \cite{caba2015activitynet}, HACS \cite{zhao2019hacs}) and Ours.}
    \label{fig:complexity}
  \end{subfigure}

  \caption{Visialisation of Dataset Analysis}
  \label{fig:TSL and complexity}
\end{figure}
