# Supplementary material for: 360+x: A Panoptic Multi-modal Scene Understanding Dataset
Source: arXiv:2404.00989 source file (2024-04-08)
Supplement: Supplementary file 11 [file datavis.tex]

% \begin{figure*}[!t]
\begin{wrapfigure}{r}{0.63\textwidth}
\begin{center}

%  左下右上
% , trim=0 0 0 0, clip
% \hspace{-1cm}

% \scalebox{0.98}{
% \begin{tabular}[b]{c} 

  % \hspace{-1cm}
  
  \includegraphics[width=0.63\textwidth ]{img/360/360_m.jpg}

% \end{tabular}
% }

\end{center}
\vspace{-2mm}
\caption{\small \textbf{Data Example of \textit{360+x}.} (a) \du circle panorama for visualizing the scene (zoom in for details). (b) The front view is extracted and undistorted from the red rectangular area of the panoramic data, where rich movement information is displayed. (c) The first-person binocular video is recorded while the wearer interacts with the scene. (d) The audio data was converted to Mel spectrograms for training. (e) The audio directional information is presented in the sound's interaural time delay.}
\label{fig:data}

\vspace{-1em}
% \end{figure*}
\end{wrapfigure}
